# Supplementary material for: Memorize and Rank: Elevating Large Language Models for Clinical Diagnosis Prediction
Source: arXiv:2501.17326 source file (2025-01-28)
Supplement: Supplementary file 1 [file 300_appendix.tex]

\reftoapp{

\vtwo{
\section{Potential Questions}

\mypar{Why not include more information, such as patient clinical notes, in the input?}
We experimented with two settings of input prompts, one with diagnosis code only and one with additional patient information as a natural language sentence. The text-code mixing input result shows that \modelname is capable of handling natural language input along with diagnosis codes. \tbref{table:diagnosis_pred_nl} shows the performance with the additional patient profile as input.

Two main reasons motivate us to use the setting of using only diagnosis codes as input for diagnosis prediction, without additional records. 
1) The setting is commonly used in existing literature (introduced in the baselines paragraph in \secref{sec:experimental_setup} and \secref{sec:relatedworks}), enabling fair head-to-head comparison with recent and state-of-the-art works. 
2) The diagnosis code-only setting is realistic for many situations where additional patient health records, such as lab test results and medical notes, are not available. Billing-related stakeholders like insurance companies only have access to diagnosis codes included in insurance filing without access to other medical records. Predicting potential future diseases is an urgently needed capability.

\mypar{How does \modelname handle missing or incomplete patient histories and data sparsity?}
For missing or incomplete data, we filter out patient records that do not have a consistent diagnosis history from our training and evaluation data. We handle the missing data in the same way as a wide range of works, many listed under the ``Baselines'' paragraph in \secref{sec:experimental_setup}.
To mitigate the influence of data sparsity, we create multiple training records from the record of a single patient described at the beginning of \secref{sec:seq2seq_data_construction}. For a patient with $T$ visits, we create $T-1$ pairs of patient history with various lengths and next-visit diagnoses. This enables us to exploit the patient records to the maximum utilization.

\mypar{Code memorization seems not to be a challenging task given almost perfect performance?}
Code memorization is not challenging only after the optimal strategy of memorizing medical code definition is found. Simply performing memorization does not work (as shown in lines 4-9 in \tbref{table:ablation_LM}). Code memorization is part of our approach to improve the diagnosis prediction capabilities, instead of the ultimate task at hand. The high performance of code memorization indicates our approach is effective. We explore different recipes to conduct code memorization in \tbref{table:ablation_LM}. We observe that 1) encoder-decoder architecture does not work for definition recall, and 2) small size model cannot memorize well. These motivate us to use decoder-only large generative language models for the diagnosis prediction task.

\mypar{Does the model compatible with encoder-only models like BERT?} We did not adapt \modelname to encoder-only models such as BERT since it would require us to remove some proposed techniques, such as intra-visit dependencies modeling.

\mypar{Is it possible to apply the method to other tasks with different output space ontology?}
The coding system $O$ to be used is an experimental setup choice. Our method design supports various coding systems. In our experiments, we show the results when using both ICD-9 (\tbref{table:diagnosis_pred_main}, \tbref{table:ablation_LM} and \tbref{table:ablation}) and ICD-10 (\tbref{table:diagnosis_pred_nl}) as the coding system.

}
}

\vtwo{
\section{Method, Implementation and Experiments Details}
\label{appendix: implementation}
\subsection{In-visit Code Order}
\label{sec:in-visit_code_order}
Though the priority among the diagnosis code list for a visit is provided in the dataset, both the MIMIC-IV dataset paper~\cite{Johnson2023MIMICIVFreelyAccessible} and dataset documentation\footnote{\url{https://mimic.mit.edu/docs/iv/modules/hosp/diagnoses_icd/#seq_num}} mentioned that there are few incentives for the operator to ensure the rank reflects the diagnosis's importance. This motivates us to train the model to ignore the order for most of the codes with perturbed code sequences.

\vthree{
\subsection{Implementation Details}

\mypar{Loss over completion only.}
Instead of language modeling where the entire sequence is used to optimize the model, we only calculate loss over the completion part assuming the input is given. For example, for definition-to-code memorization, we only apply loss to let the model output the correct code. We do not apply the next token prediction for the question part and do not require the model to learn to reconstruct the question ``What is the ICD-9 code with the definition ...''.

\mypar{Getting top-k predictions from free-text responses.} The LM will general responses as an output sequence; we then parse the output sequence to a set of diagnosis codes separately by white space. The LM decides the number of predictions made by the LM. 
When calculating metrics like recall@20 and the number of prediction codes is less than 20 codes, we do not force the model to generate more codes.

\subsection{Experimental Setup Details}
\label{appendix:experimental_setup_details}
We use the records of patients having multiple visits and use the complete medical code to represent the diagnosis. This poses a more challenging task compared to some existing studies that use simplified and higher-level codes. To prevent data duplication within the overlapping time frame of the two datasets, only the patient information from MIMIC-IV with multiple visits between 2013 and 2019 was used. 
In the validation and test sets, we designate the patients' last visit as the label for prediction, with the preceding visit(s) used to construct input.

For the settings using ICD-10 as decision space, we use a subset of patients in the MIMIC-IV dataset whose diagnosis records are all in ICD-10 to avoid potential errors during code version conversion. Records of 4277 patients are used for training, and the remaining 500 are used for evaluation. The input of this setting would be a sequence of ICD-10 codes, and the expected diagnoses to be predicted are also selected from a list of all ICD-10 codes.

We show the data statistics of the training and evaluation data used in our experiments in \tbref{table:data_stats}.
}

\begin{table}[h]
\begin{center}
{
\small
\begin{tabular}{l|rr}
\toprule
Dataset & MIMIC-III & MIMIC-IV 
\\ \midrule
\# unique patients & 7493 & 10000 
\\
Train/valid/test splits & 6000/493/1000 & 8000/1000/1000
\\
Max. \# visit & 42 & 55
\\
Avg. \# visit & 2.66 & 3.66
\\ \hline
\# unique diagnosis codes & 4880 & 6102 
\\
Max. \# codes per visit & 39 & 50
\\
Avg. \# codes per visit & 13.06 & 13.38
\\
\bottomrule
\end{tabular}
}
\end{center}
\caption{
Data statistics.
}
\label{table:data_stats}
\end{table}

\reftoapp{
\subsection{Baseline Details}
\label{appendix:baseline_details}
\mypar{RNN/CNN and attention-based models.}
\textbf{RETAIN} \cite{Choi2016RETAINInterpretablePredictive} employs two attention mechanisms to model two-way visit-disease mapping. 
\textbf{Dipole}~\cite{Ma2017DipoleDiagnosisPredictionb} proposes a bidirectional RNN to address the issue of lengthy medical visit records. \textbf{Timeline}~\cite{Bai2018InterpretableRepresentationLearning} designs an attention mechanism that combines time intervals and attention weights of each entity. \textbf{HiTANet}~\cite{Luo2020HiTANetHierarchicalTimeAware} employs a hierarchical temporal attention mechanism. \textbf{Deepr}~\cite{Nguyen2017MathttDeeprConvolutional} predicts future risks from medical records by converting records into discrete element sequences and using a CNN to detect predictive local clinical patterns.

\mypar{Graph-based models.}
\textbf{GRAM}~\cite{Choi2017GRAMGraphbasedAttention} employs the structure of medical ontologies. \textbf{G-BERT}~\cite{Shang2019PretrainingGraphAugmented} integrates pretrained language models and considers the hierarchical information of ICD codes. \textbf{CGL}~\cite{Lu2021CollaborativeGraphLearning} introduces a collaborative graph learning model. \textbf{Chet}~\cite{Lu2022ContextAwareHealthEvent} computes the diagnosis neighbor and global neighbor for each disease. \textbf{MCDP}~\cite{Li2022MultimodalContrastiveLearning} uses hyperbolic space to preserve the hierarchical structure of diagnostic codes. 
\textbf{KGxDP}~\cite{Yang2023InterpretableDiseasePrediction} formulates each patient as a personalized medical KG, combining medical KGs with patient admission history. Note that additional medical notes are used by CGL, and additional Unified Medical Language System resource~\cite{bodenreider2004unified} is used as external knowledge by KGxDP. 

We cannot reproduce MCDP~\cite{Li2022MultimodalContrastiveLearning}, so we only report results in the paper.
}

}

\reftoapp{
\subsection{Computational Complexity}
\label{appendix: computation}
We perform full parameter supervised fine-tuning without using any parameter-efficient training techniques as we observe that full parameter tuning leads to better performance. We use 4 A6000 GPUs for an average of 53 hours to train our model (line 15 of \tbref{table:diagnosis_pred_main}) until the validation F1 score does not improve.
}

\section{Complete Prompt Example}
\label{sec:complete_prompt}

We show an exemplar input and output for the diagnosis prediction task. The green background segment is the output sequence. All the token that starts with ``ICD9\_'' are special tokens that would map to a unique token representation. \texttt{EOV} is also a special token representing the end of a hospital visit.

\begin{tcolorbox} 
    \centering
    \begin{tabular}{p{0.97\columnwidth} c}
    \footnotesize
    
    The task is to predict the diagnosis codes for the next patient visit given the patient diagnosis history.

    \#\#\# Patient history: 
    Diagnosis codes for the visit: ICD9\_443.9 ICD9\_785.4 ICD9\_585.9 ICD9\_584.9 ICD9\_250.70 ICD9\_250.60 ICD9\_357.2 ICD9\_369.4 ICD9\_403.90 ICD9\_V58.67 ICD9\_V12.59 \texttt{EOV} Diagnosis codes for the visit: ICD9\_584.9 ICD9\_427.5 ICD9\_348.30 ICD9\_276.2 ICD9\_403.11 ICD9\_428.22 ICD9\_250.80 ICD9\_428.0 ICD9\_585.6 ICD9\_790.4 ICD9\_787.01 ICD9\_285.21 ICD9\_272.4 ICD9\_782.3 ICD9\_786.6 ICD9\_794.31 ICD9\_607.9 ICD9\_608.9 ICD9\_564.00 ICD9\_V58.67 ICD9\_E932.3 ICD9\_V02.54 \texttt{EOV}
    
    \#\#\# Diagnosis for the next visit: \\
    \colorbox{green!30}{
    ICD9\_038.9 ICD9\_585.6 ICD9\_403.91 ICD9\_428.20 ICD9\_276.2 ICD9\_995.91
    }
    \colorbox{green!30}{ICD9\_608.83 ICD9\_428.0 \texttt{EOV}
    }
    \end{tabular}
\end{tcolorbox}

\vtwo{
\section{Limitations}
\label{appendix: limitation}
We would like to raise awareness that there might be miscoded diagnosis codes in the patient records. The billing ICD diagnosis codes are used as “ground-truth” diagnosis decisions to train our model and evaluate the performance for diagnosis prediction. We acknowledge that the diagnosis code extracted from the EHR dataset should not be considered the best/perfect diagnosis decision. We also raise the potential data distribution issue as the training and evaluation data used in this work is largely collected for patients with ICU stay history. Thus, the evaluation result does not represent the generalized diagnosis prediction capability, and the trained model may yield compromised performance when different kinds of patient records are queried.
\section{Ethical Statement}
\label{appendix: ethics}
While \modelname demonstrates improved performance in diagnostic prediction tasks, the trained model may incorporate biases from multiple sources, including the pre-training corpus or the medical records distribution utilized for fine-tuning, and more. Therefore, the model necessitates comprehensive evaluation prior to its consideration for real-world clinical application. Additionally, the outcomes of the diagnostic prediction model may not be utilized to attribute discriminatory labels to specific diseases. Healthcare institutions and insurance entities may not use the predictive diagnoses of \modelname as a basis for changing patient services.
\section{Broader Impact Statement}
\label{appendix: impact}
\modelname contributes to the potential improvement of healthcare delivery and patient outcomes. By aiming to accurately predict diseases based on patient medical histories, these models offer a possibility for earlier detection and intervention, which might lead to better patient outcomes over time. Given the challenges associated with limited patient data and the complexity of diagnosing a wide range of diseases, \modelname's approach, which leverages Large Language Models (LLMs) and hierarchical contrastive learning, represents a step towards addressing these issues. While its performance on the MIMIC datasets indicates promising results in diagnosis prediction, the real-world application of such models underscores the cautious optimism for AI's role in enhancing clinical decisions and healthcare efficiency. These developments suggest a direction where AI could support more informed clinical decisions, potentially improving patient care and management, albeit with ongoing evaluation and validation needed to fully realize these benefits.

}
